# Supplementary material for: Finding Adversarial Inputs for Heuristics using Multi-level Optimization
Source: arXiv:2311.12779 source file (2023-11-21)
Supplement: Supplementary file 1 [file appendix.tex]

\appendix
%\section*{Appendix}

%\renewcommand{\thesubsection}{\Alph{subsection}}
\setcounter{subsection}{0}
\setcounter{section}{0}
\setcounter{figure}{0}
\setcounter{table}{0}

\section{Detailed mathematical formulations and proofs}
\subsection{Multi-commodity flow problem}
\label{sec::appendix-flow}

The optimal form of WAN-TE typically involves solving a multi-commodity flow problem. Given a set of nodes, capacitated edges, demands, and pre-chosen paths per demand, a flow allocation is feasible if it satisfies demand and capacity constraints. The goal is to find a feasible flow to optimize a given objective (e.g., total flow~\cite{ncflow}, max-min fairness~\cite{swan,b4}, or utility curves~\cite{bwe}). We define the feasible flow over a pre-configured set of paths as (see Table~\ref{t:notation})

\vspace{-3mm}
{\footnotesize
	\begin{alignat}{4}
	&\multispan{4}\mbox{$\displaystyle \label{eq:feasible_flow} {\sf FeasibleFlow}(\mathcal{V}, \mathcal{E}, \mathcal{D}, \mathcal{P}) \triangleq \big\{\mathbf{f} \mid$}&\\
	&f_k = \sum_{p \in \mathcal{P}_k} f_k^p, & \forall k \in \mathcal{D} & \quad \text{(flow for demand $k$)}\nonumber\\
	&f_k \leq d_k, & \forall k \in \mathcal{D} & \quad \text{(flow below volume)}\nonumber\\
	&\sum_{k, p \mid p \in \mathcal{P}_k, e \in p} \!\!\!\!\! f_k^p \leq c_e, & \forall e \in \mathcal{E} & \quad \text{(flow below capacity)}\nonumber\\
	&f_k^p \geq 0 & \forall p \in \mathcal{P}, k \in \mathcal{D} & \quad \text{(non-negative flow)}\big\}\nonumber
	\end{alignat}}
Among all the feasible flows, the optimal solution seeks to maximize the total flow across the network:

\vspace{-3mm}
{\footnotesize
	\begin{align}
	\label{eq:max_flow}
	\mbox{\sf OptMaxFlow}(\mathcal{V}, \mathcal{E}, \mathcal{D}, \mathcal{P}) \triangleq & \arg\max_{\mathbf{f}}\sum_{k \in \mathcal{D}} f_k\\
	\mbox{s.t.} \quad & \mathbf{f} \in {\sf FeasibleFlow}(\mathcal{V}, \mathcal{E}, \mathcal{D}, \mathcal{P}).\nonumber
	\end{align}}

%Variables and constraints of optimization \eqref{eq:max_flow} increase with $|\mathcal{D}| + |\mathcal{E}|$ where $|\mathcal{D}|$ is typically quadratic in $|\mathcal{V}|$. 
%Prior work shows this does not scale: at large network sizes, the solver can take tens of minutes to finish, which hinders its use in practice for managing networks with dynamic demands~\cite{ncflow}. 

\subsection{{\pop} Client Splitting}
\label{s:appendix:pop}

In~\secref{s:background}, we introduce the (basic) \pop heuristic~\cite{pop}, which incorporates \emph{resource splitting} for our WAN TE problem, and in~\secref{ss:convexify}, we argue that \pop can be represented as a convex optimization problem.
The work in~\cite{pop} also specifies an extended full-fleshed version of the heuristic that incorporates an additional operation named \emph{client splitting}.
In this appendix, we demonstrate that the extended version of \pop can also be expressed as a convex optimization problem.

We can think of \pop client splitting as an operation that takes in a set of demands $\mathcal{D}$ and returns a modified set $\mathcal{D}_{\mathrm{cs}} = \mathrm{ClientSplit}(\mathcal{D})$ that can then be input into \pop as in~\eqref{eq:pop_max_flow}.
The function $\mathrm{ClientSplit}()$ generates several duplicates of the existing demands and reduces their volume accordingly. In essence, it performs several operations where $(s_k, t_k, d_k) \in \mathcal{D}$ is replaced by two elements of the form $(s_k, t_k, d_k/2)$.
This operation is iteratively performed until the process is terminated; see~\cite{pop} for more details.

%~\cite{pop} pre-specifies the total number of splits among all clients. We slightly modify this in order to facilitate modeling the problem in convex form. Specifically, we convert the total number for splits to a per-client budget and constrain the number of splits for each client: this {\em may} result in slightly worse optimality gap, as this encoding of the heuristic is strictly contained in the solution space of~\cite{pop}.

Below we propose a way to encode a version client splitting where we split an element in $\mathcal{D}$ if its demand value $d_k$ is larger than or equal to a threshold $d_{\mathrm{th}}$, and we keep splitting it until either we get to a predefined number of maximum splits of the original demand\footnote{Notice that~\cite{pop} pre-specifies a total aggregated number of splits across all clients whereas we set the a maximum for per-client splits. This slight modification facilitates the convex representation of the heuristic.} or the split demand is lower than $d_{\mathrm{th}}$.

Without loss of generality, we illustrate this idea for a single demand $d_1$: we can replicate this process for all demands in $\mathcal{D}$.
For concreteness, let us set that we will split this demand at most twice (giving rise to at most $4$ virtual clients).
Hence, we construct a priori the flows for all the possible splits of the client $d_1$.
More precisely, instead of having a single variable $f_1$ for the first demand (see~\autoref{t:notation}) we have seven variables where $f_{1,1}$ is the flow if we do not split the client, $f_{1,2}$ and $f_{1,3}$ are the flows if we split the client once, and $f_{1,4}$ through $f_{1,7}$ are the flows if we split the client twice. 
Notice that these flows must satisfy the following linear constraints
\begin{align*}
	0 & \leq f_{1,1} \leq d_1, \\
	0 & \leq f_{1,i} \leq \frac{d_1}{2}, \,\,\, \text{for } i \in \{2, 3\} \\
	0 &\leq f_{1,i} \leq \frac{d_1}{4},  \,\,\, \text{for } i \in \{4, 5, 6, 7\}. 
\end{align*}
Now, we want $f_{1,1}$ to be exactly zero unless $d_1 < d_{\mathrm{th}}$ (hence, no client splitting occurs), which we can achieve using big-$M$ constraints as illustrated in~\secref{ss:convexify}, i.e.,
\begin{align*}
	f_{1,1} \leq \max( M (d_{\mathrm{th}}-d_1), 0).
\end{align*}
Similarly, we want $f_{1,2}$ and $f_{1,3}$ to be exactly zero unless $d_1 \geq d_{\mathrm{th}}$ and $d_1/2 < d_{\mathrm{th}}$, which we can achieve by doing
\begin{align*}
	f_{1,i} & \leq \max( M (d_1-d_{\mathrm{th}}+\epsilon), 0),  && \,\,\, \text{for } i \in \{2, 3\}, \\
	f_{1,i} & \leq \max( M (d_{\mathrm{th}}-d_1/2), 0),  && \,\,\, \text{for } i \in \{2, 3\},
\end{align*}
where the small pre-specified $\epsilon >0$ is added to allow for the case where $d_1 = d_{\mathrm{th}}$.
Lastly, we want $f_{1,4}$ through $f_{1,7}$ to be exactly zero unless $d_1 \geq 2 d_{\mathrm{th}}$.
This can be encoded as
\begin{align*}
	f_{1,i} & \leq \max( M (d_1-2d_{\mathrm{th}}+\epsilon), 0),  && \,\,\, \text{for } i \in \{4, 5, 6, 7\}.
\end{align*}
The procedure here illustrated for the first demand can be replicated for all $d_k$, thus effectively encoding \pop with client splitting as a convex optimization problem. Once this is done, the techniques in~\secref{s:methods} apply.

\iffalse
\fi

\subsection{Demand Pinning Big-$M$ form}
\label{sec:dempin_bigM}

We can also encode \dempin using the standard big-$M$ approach from optimization theory~---~we need this for the KKT-encoding where we do not have quantized demands.

We describe the shortest path for demand $k$ using $\widehat{p}_k$ and write the {\em if} clause as:

{\small
	\begin{eqnarray}
	\sum_{p \in P_k,\ p \neq \widehat{p}_k} f_k^p \leq \max\left(M(d_k - T_d), 0\right), \,\,\, \forall k \in \mathcal{D}, \nonumber \\
	d_k - f_k^{\widehat{p}_k} \leq \max\left(M(d_k - T_d), 0\right), \,\,\, \forall k \in \mathcal{D}, \nonumber
	\end{eqnarray}
}
where $M$ is a large pre-specified constant.
Notice whenever the demand $d_k$ is below the threshold $T_d$ the constraints allocate zero flow on all but the (default) shortest path~---~\dempin routes the {\em full demand} on the default path in such cases. We can use standard optimization theory to convert the $\max$ in these constraints into a set of linear constraints~\cite{boyd_co} (the change also requires we modify the objective but does not impact the quality of the solution).

\subsection{First Fit Decreasing formulation}
\label{sec:vbp_details}

The various weight functions researchers have proposed in \vbp are:

{\small 
	\begin{alignat}{3}
	FFDSum(Y^i) \triangleq & \sum\limits_{d=1}^{n}{Y^d_i} & \nonumber\\
	FFDProd(Y^i) \triangleq & \Pi_{d=1}^{n}{Y^d_i} & \nonumber\\ 
	FFDDiv(Y^i) \triangleq & \frac{Y^j_1}{Y^j_2} & \mbox{(only 2-dimension)} \nonumber
	\end{alignat}
}
where $Y^d_i$ is the size of item $i$ in dimension $d$.

In each iteration, \ffd finds the largest un-assigned ball. We can model this naively using a sorting network~\cite{sorting_net_1} and sort the balls to find the largest one. But this limits our ability to scale. We instead leverage the inherent symmetry of the problem~---~we only need to consider a pre-sorted set of ball sizes because for every ordering of ball sizes there exists a sorted ordering with the same allocation from \ffd. 
\behnaz{@Pooria I did not at all parse what you were trying to say in this last sentence so I had to leave it as is, please try to clarify.}
~---~and use the ${\sf ConstrainedSet}$ in \eqnref{eq:metaopt_full} to make sure {\metaopt} only considers cases where the balls are already sorted;
{\small
	\begin{equation}
	w_{i} \geq w_{i + 1} \,\,\, \forall{\sf item}\,\, i \nonumber
	\end{equation}
}
where $w_{i}$ is the weight of item $i$ based on {\ffd} function (\eg FFDSum).

We next need to model how \ffd places the item $i$ in the first available bin with enough capacity. We use auxilary binary variables $\beta_{ij}$ that specify whether item $i$ fits in bin $j$ ($\beta_{ij} = 1$ if it does not fit) and find the first bin with $\beta_{ij = 0}$:

{\small 
	\begin{alignat}{3}
	\sum\limits_{j}\alpha_{ij} & = 1 & ~~~\forall{\sf item}\,{i} \nonumber \\
	\alpha_{ij} & \leq \frac{1 -\beta_{ij} + \sum_{k=1}^{j - 1}{\beta_{ik}}}{j} & ~~~\forall{\sf item}\, i \,\,\forall{\sf bin}\, j \nonumber
	\end{alignat}
}
where $\alpha_{ij}$ indicates whether we place item $i$ in bin $j$. The first constraint ensures we do not assign an item more than once and the second ensures we place the item in the first bin with enough capacity: the right hand side is less than one in all cases where an earlier bin has capacity and forces $\alpha_{ij}$ to zero in such cases.

We next need to model whether item $i$ fits in bin $j$ on all dimension: we need to measure for each bin $j$ how much capacity remains for each dimension $d$ after we place balls $\{0,1,\dots i-1\}$. We add one variable per item per bin, $x^d_{ij}$, that measures how of bin $j$'s capacity in dimension $d$ ball $i$ uses. The $x^d_{ij}$ for item $i$ are non-zero for only a single bin and equal to the size of the item:

{\small
	\begin{alignat}{3}
	x^{d}_{ij} & \leq M_1 \alpha_{ij} & ~~~\forall {\sf item}\, i \,\,\forall {\sf bin}\, j \,\,\forall {\sf dim}\, {d}\nonumber \\
	\sum_{j} x_{ij}^d & = Y^{d}_{i} & ~~~ \forall{\sf item}\, i \,\,\forall {\sf dim}\, {d}\nonumber
	\end{alignat}
}

where $M_1$ is a large constant and an upper bound on $Y^d_i$. We then use $x^d_{ij}$ to measure whether remaining capacity of the $d$-th dimension of bin $j$ is enough to fit ball $i$ (shown by a binary variable $\beta^d_{ij}$ which is $=1$ if does not fit):
{\small
	\begin{alignat}{3}
	- M_2 \beta_{ij}^{d} & \leq C_j^d - Y_i^d - \sum_{u=1}^{i-1} x_{uj}^d & ~~~\forall {\sf item}\, i \,\,\forall \,\,{\sf bin}\, j \,\,\forall {\sf dim}\, {d} \nonumber \\
	M_2(1 - \beta_{ij}^d) & \geq C_j^d - Y_i^d - \sum_{u=1}^{i-1} x_{uj}^d + \epsilon & ~~~\forall {\sf item}\, i \,\,\forall {\sf bin}\, j \,\,\forall {\sf dim}\, {d} \nonumber
	\end{alignat}
}
where $C^d_j$ is the capacity of the $d$-th dimension of bin $j$, $M_2$ is a large constant and an upper bound on $C^d_j$ and $\epsilon$ is a small positive constant.

An item $i$ only fits in bin $j$ if all of its dimensions fit ($\exists d: \beta^d_{ij} = 1$);
{\small
	\begin{alignat}{3}
	\beta_{ij} & \geq \beta_{ij}^d & ~~~\forall {\sf item}\, i \,\,\forall {\sf bin}\, j \,\,\forall {\sf dim}\, {d}\nonumber \\
	\beta_{ij} & \leq \sum_{d}\beta^{d}_{ij} & ~~~\forall{\sf item}\, i \,\,\forall{\sf bin}\, j \nonumber
	\end{alignat}
}

We now need to specify the leader's payoff. \ffd's goal is to minimize the number of bins it uses: it maximizes $-\sum_{j}{P_{j}}$ where $P_{j}$ is a binary variable that shows whether we use bin $j$

{\small
	\begin{alignat}{3}
	P_{j} & \geq \alpha_{ij} & ~~~\forall{\sf item}\, i \,\,\forall{\sf bin}\, j \nonumber \\
	P_{j} & \leq \sum_{i} \alpha_{ij} & ~~~\forall{\sf bin}\, j \nonumber 
	\end{alignat}
}
The first constraint requires $P_{j} = 1$ if there is at least one item placed in the bin ($\exists i: \, \alpha_{ij} = 1$), and the second constraint ensures $P_{j} = 0$ if the bin is completely empty ($\forall i: \, \alpha_{ij} = 0$). 

\pooria{we need to add a table with description of all the variables}

\subsection{Proof of \theoremref{th:ffdsum:approx-ratio}}
\label{apendix:proof:ffdsum}
\pooria{will complete this.}

\section{Black-box search methods}
\label{appendix:black-box}
\pooria{will make a pass over this to make sure it is consistent.}
\parae{Random search.} We compare \metaopt to a simple (strawman) random search solution: the solution picks random inputs, computes the gap, and returns the input that resulted in the maximum gap after .

\parae{Hill climbing} is arguably the simplest local search algorithm. It first randomly chooses an arbitrary input $\mathbf{d}_0$ and generates neighbors: it adds a value, which it draws from a zero-mean  $\sigma^2$-variance Gaussian distribution, independently to each element of the current input. If this neighboring input increases the gap the hill climber moves to that input. Otherwise it draws another neighbor. The hill climber repeats these steps until it terminates.

The hill climber terminates and outputs the current solution as the local maximum (Algorithm~\ref{alg:hc}) if it does not find an input that increases the gap in $K$ consecutive rounds. 

We re-run the hill climber $M_\mathrm{hc}$ times with different initial inputs and return the solution that produces the maximum gap to minimize the impact of the starting point.

In our evaluations: $\sigma=10\%$ of link capacity, $K=100$ and $M_\mathrm{hc}$ based on the latency budget.

\begin{algorithm}[t]
	\caption{Hill climbing}\label{alg:hc}
	\begin{algorithmic}
		\begin{footnotesize}
			\Input : $\mathbf{d}_0$, $\sigma^2$, $K$
			\EndInput
			\State $\mathbf{d} \gets \mathbf{d}_0$, $\,\,\,k \gets 0$ 
			\While{$k < K$}
			\State $\mathbf{d}_{\mathrm{aux}} \gets \max(\mathbf{d} + \mathbf{z}, \mathbf{0})\,\,\,\,$ where $\,\,\,\,\mathbf{z} \sim \mathcal{N} (\mathbf{0}, \sigma^2 \mathbf{I})$
			\IIf{$\mathrm{gap}(\mathbf{d}_{\mathrm{aux}})>\mathrm{gap}(\mathbf{d})$} $\mathbf{d} \gets \mathbf{d}_{\mathrm{aux}}$, $\,\,\,k \gets -1$
			\EndIIf
			\State $k \gets k+1$			
			\EndWhile
			\Output : $\mathbf{d}$
			\EndOutput
		\end{footnotesize}
	\end{algorithmic}
	\vspace{-1mm}
\end{algorithm}

\parae{Simulated annealing} refines hill-climbing and seeks to avoid getting trapped in a local maxima~\cite{simulated_annealing}. The difference between the two algorithms is that simulated annealing may still (with some probability) move to a neighboring input even if that input does not improve the gap.

\behnaz{@Pooria you never defined $d_{aux}$}

Simulated annealing gradually decreases the probability of moving to inputs that do not change the gap: it defines a temperature term, $t_p$, which it decreases every $K_p$ iterations to $t_{p+1} = \gamma t_{p}$. Here, $0<\gamma <1$ which ensures $t_p \to 0$. If~$\mathrm{gap}(\mathbf{d}_{\mathrm{aux}}) \leq \mathrm{gap}(\mathbf{d})$, we have $\mathbf{d} \gets \mathbf{d}_{\mathrm{aux}}$ with probability $\exp(\frac{\mathrm{gap}(\mathbf{d}_{\mathrm{aux}}) - \mathrm{gap}(\mathbf{d})}{t_p})$.

%$t_p$ is initialized at $t_0$, and in every $K_p$ iterations, it is decreased as $t_{p+1} = \gamma t_{p}$ for $0<\gamma <1$.
%Notice that $t_p \to 0$, i.e., the probability of moving to a demand that does not improve the gap decreases with iterations. Thus, simulated annealing mimics hill climbing more closely as the number of iterations increases.
We repeat the process $M_{\mathrm{sa}}$ times and return the best solution. We initialize $t_p$ to $t_0=500$, and set $\gamma=0.1$, $K_p=100$, and $M_{\mathrm{sa}}$ based on what latency we require.

\parae{Hill climbing vs simulated annealing.} Hill climbing has less parameters and is better suited for smooth optimizations where there are few local-optima. But simulated annealing is better suited for intricate non-convex optimizations with many local-optima because its exploration phase, although slower, allows it to avoid local optima and works better in the long run.

Both of these algorithms have a number of hyperparameters: we run grid-search to find the ones that produce the highest gap.
