# Supplementary material for: Finding Adversarial Inputs for Heuristics using Multi-level Optimization
Source: arXiv:2311.12779 source file (2023-11-21)
Supplement: Supplementary file 3 [file appendix_ffd_old.tex]

\subsection{First Fit Decreasing formulation}
\label{sec:vbp_details}

The various weight functions researchers have proposed in \vbp are:

{\small 
	\begin{alignat}{3}
		FFDSum(Y^i) \triangleq & \sum\limits_{d=1}^{n}{Y^d_i} & \nonumber\\
		FFDProd(Y^i) \triangleq & \Pi_{d=1}^{n}{Y^d_i} & \nonumber\\ 
		FFDDiv(Y^i) \triangleq & \frac{Y^j_1}{Y^j_2} & \mbox{(only 2-dimension)} \nonumber
	\end{alignat}
}
where $Y^d_i$ is the size of item $i$ in dimension $d$. 


In each iteration, \ffd finds the largest un-assigned ball. We can model this naively using a sorting network~\cite{sorting_net_1} and sort the balls to find the largest one. But this limits our ability to scale. We instead leverage the inherent symmetry of the problem~---~we only need to consider a pre-sorted set of ball sizes because for every ordering of ball sizes there exists a sorted ordering with the same allocation from \ffd. 
\behnaz{@Pooria I did not at all parse what you were trying to say in this last sentence so I had to leave it as is, please try to clarify.}
~---~and use the ${\sf ConstrainedSet}$ in \eqnref{eq:metaopt_full} to make sure {\metaopt} only considers cases where the balls are already sorted;
{\small
	\begin{equation}
		w_{i} \geq w_{i + 1} \,\,\, \forall{\sf item}\,\, i \nonumber
	\end{equation}
}
where $w_{i}$ is the weight of item $i$ based on {\ffd} function (\eg FFDSum).

We next need to model how \ffd places the item $i$ in the first available bin with enough capacity. We use auxilary binary variables $\beta_{ij}$ that specify whether item $i$ fits in bin $j$ ($\beta_{ij} = 1$ if it does not fit) and find the first bin with $\beta_{ij = 0}$:


{\small 
	\begin{alignat}{3}
		\sum\limits_{j}\alpha_{ij} & = 1 & ~~~\forall{\sf item}\,{i} \nonumber \\
		\alpha_{ij} & \leq \frac{1 -\beta_{ij} + \sum_{k=1}^{j - 1}{\beta_{ik}}}{j} & ~~~\forall{\sf item}\, i \,\,\forall{\sf bin}\, j \nonumber
	\end{alignat}
}
where $\alpha_{ij}$ indicates whether we place item $i$ in bin $j$. The first constraint ensures we do not assign an item more than once and the second ensures we place the item in the first bin with enough capacity: the right hand side is less than one in all cases where an earlier bin has capacity and forces $\alpha_{ij}$ to zero in such cases.

We next need to model whether item $i$ fits in bin $j$ on all dimension: we need to measure for each bin $j$ how much capacity remains for each dimension $d$ after we place balls $\{0,1,\dots i-1\}$. We add one variable per item per bin, $x^d_{ij}$, that measures how of bin $j$'s capacity in dimension $d$ ball $i$ uses. The $x^d_{ij}$ for item $i$ are non-zero for only a single bin and equal to the size of the item:


{\small
	\begin{alignat}{3}
		x^{d}_{ij} & \leq M_1 \alpha_{ij} & ~~~\forall {\sf item}\, i \,\,\forall {\sf bin}\, j \,\,\forall {\sf dim}\, {d}\nonumber \\
		\sum_{j} x_{ij}^d & = Y^{d}_{i} & ~~~ \forall{\sf item}\, i \,\,\forall {\sf dim}\, {d}\nonumber
	\end{alignat}
}


where $M_1$ is a large constant and an upper bound on $Y^d_i$. We then use $x^d_{ij}$ to measure whether remaining capacity of the $d$-th dimension of bin $j$ is enough to fit ball $i$ (shown by a binary variable $\beta^d_{ij}$ which is $=1$ if does not fit):
{\small
	\begin{alignat}{3}
		- M_2 \beta_{ij}^{d} & \leq C_j^d - Y_i^d - \sum_{u=1}^{i-1} x_{uj}^d & ~~~\forall {\sf item}\, i \,\,\forall \,\,{\sf bin}\, j \,\,\forall {\sf dim}\, {d} \nonumber \\
		M_2(1 - \beta_{ij}^d) & \geq C_j^d - Y_i^d - \sum_{u=1}^{i-1} x_{uj}^d + \epsilon & ~~~\forall {\sf item}\, i \,\,\forall {\sf bin}\, j \,\,\forall {\sf dim}\, {d} \nonumber
	\end{alignat}
}
where $C^d_j$ is the capacity of the $d$-th dimension of bin $j$, $M_2$ is a large constant and an upper bound on $C^d_j$ and $\epsilon$ is a small positive constant.

An item $i$ only fits in bin $j$ if all of its dimensions fit ($\exists d: \beta^d_{ij} = 1$);
{\small
	\begin{alignat}{3}
		\beta_{ij} & \geq \beta_{ij}^d & ~~~\forall {\sf item}\, i \,\,\forall {\sf bin}\, j \,\,\forall {\sf dim}\, {d}\nonumber \\
		\beta_{ij} & \leq \sum_{d}\beta^{d}_{ij} & ~~~\forall{\sf item}\, i \,\,\forall{\sf bin}\, j \nonumber
	\end{alignat}
}

We now need to specify the leader's payoff. \ffd's goal is to minimize the number of bins it uses: it maximizes $-\sum_{j}{P_{j}}$ where $P_{j}$ is a binary variable that shows whether we use bin $j$

{\small
	\begin{alignat}{3}
		P_{j} & \geq \alpha_{ij} & ~~~\forall{\sf item}\, i \,\,\forall{\sf bin}\, j \nonumber \\
		P_{j} & \leq \sum_{i} \alpha_{ij} & ~~~\forall{\sf bin}\, j \nonumber 
	\end{alignat}
}
The first constraint requires $P_{j} = 1$ if there is at least one item placed in the bin ($\exists i: \, \alpha_{ij} = 1$), and the second constraint ensures $P_{j} = 0$ if the bin is completely empty ($\forall i: \, \alpha_{ij} = 0$). 

\pooria{we need to add a table with description of all the variables}
